# Supplementary material for: An information-theoretic perspective on intrinsic motivation in reinforcement learning: a survey
Source: arXiv:2209.08890 source file (2022-09-19)
Supplement: Supplementary file 1 [file appendixes.tex]

\appendix
\appendixpage
\section{Intrinsic motivation and other forms of learning}\label{append:distinction}

Table \ref{tab:rlim} shows the difference between reinforcement learning and the use of IM. Reinforcement learning is an active process since the agent learns from its interactions with the environment, unlike classification or regression which are supervised methods. Unsupervised learning is a passive learning process, \textit{i.e.} it does not use predefined labels, or in other words, learns without a feedback. Finally, the substitution of the feedback by an intrinsic reward allows to break free from an expert supervision; however, the difference remains between IM and unsupervised learning in the sense that IM is an active process which implies interactions.

\begin{table}[t]
\centering

 \caption{Type of learning. \textit{feedback} here refers to an expert supervision.}\label{tab:rlim}
\begin{tabular}{|l|l|l|}
  \hline
   & With \textit{feedback}  & Without \textit{feedback} \\
  \hline
    Active & Reinforcement & Intrinsic motivation \\
    Passive & Supervised & Unsupervised \\
  \hline

\end{tabular}
\end{table}

\section{Challenges of RL tackled with IM}\label{sect:defis}

%In this section, we detail the main challenges of reinforcement learning that can be addressed with intrinsic motivation. 
In this section, we identify four challenges in DRL for which IM provides a suitable solution. We illustrate these challenges and explain their importance.

%\subsection{RL problematic}\label{sect:defis}
\subsection{Sparse rewards} 

Classic RL algorithms operate in environments where the rewards are \textbf{dense}, \textit{i.e.} the agent receives a reward after almost every completed action. In this kind of environment, naive exploration policies such as $\epsilon$-greedy \cite{sutton1998reinforcement} or the addition of a Gaussian noise on the action \cite{lillicrap2015continuous} are effective. More elaborated methods can also be used to promote exploration, such as Boltzmann exploration \cite{cesa2017boltzmann,mnih2015human}, an exploration in the parameter-space \cite{plappert2017parameter,ruckstiess2010exploring,fortunato2017noisy} or Bayesian RL \cite{ghavamzadeh2015bayesian}. In environments with \textbf{sparse} rewards, the agent receives a reward signal only after it executed a large sequence of specific actions. The game \textit{Montezuma's revenge} \cite{bellemare15} is a benchmark illustrating a typical sparse reward function. In this game, an agent has to move between different rooms while picking up objects (it can be keys to open doors, torches, ...). The agent receives a reward only when it finds objects or when it reaches the exit of the room. Such environments with sparse rewards are almost impossible to solve with the above mentioned exploration policies since the agent does not have local indications on the way to improve its policy. Thus the agent never finds rewards and cannot learn a good policy with respect to the task \cite{mnih2015human}. Figure \ref{im:sparse_reward} illustrates the issue on a simple environment.% where the agent strives to find a star. 
\begin{figure}
\begin{centering}
\includegraphics[width=10cm]{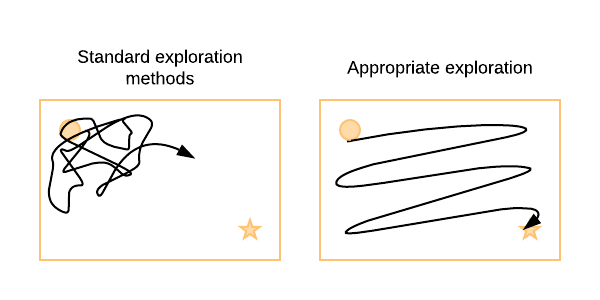}
\caption{Illustration of the sparse reward issue in a very simple setting. The agent, represented by a circle, strives to reach the star. The reward function is one when the agent reaches the star and zero otherwise. On the left side, the agent explores with standard methods such as $\epsilon-greedy$; as a result, it stays in its surrounded area because of the temporal inconsistency of its behaviour. On the right side, we can imagine an ideal exploration strategie where the agent covers the whole state space to discover where rewards are located.}
\label{im:sparse_reward}
\end{centering}
\end{figure}

Rather than working on an exploration policy, it is common to shape an intermediary dense reward function which adds to the reward associated to the task in order to make the learning process easier for the agent \cite{su2015reward}. However, the building of a reward function often reveals several unexpected errors \cite{ng1999policy,amodei2016concrete} and most of the time requires expert knowledge. For example, it may be difficult to shape a local reward for navigation tasks. Indeed, one has to be able to compute the shortest path between the agent and its goal, which is the same as solving the navigation problem. On the other side, the automation of the shaping of the local reward (without calling on an expert) requires too high computational resources \cite{chiang2019learning}.

We will see in \S\ref{curiosity} how IM is a valuable method to encourage exploration in a sparse rewards setting. In \S\ref{sec:curriculum}, we also provide details on the value of IM in the context of\textit{curriculum learning}for exploration.

%--P3
\subsection{Building a good state representation}\label{sec:staterepresentation}

What is a good state representation? \citename{bohmer2015autonomous} argue that, in standard RL, this representation must be markovian, able to represent the true value of the policy, generalize well and low-dimensional. Using such adapted feature space to learn a task can considerably accelerate the learning process \cite{raffin2019decoupling,de2018integrating} and may even help with other computations such as learning a forward model. The best way to do this may be to construct a minimal feature space with \textbf{disentangle features} \cite{bengio2013representation,lesort2018state}. 

In order to better understand the importance of a relevant state representation in RL, let us consider a simple navigation task where the agent has to reach a target area in an empty space. If the agent accesses pixels input from above, it will have to extract its own position and the target position through complex non-linear transformations to understand which directions it has to take. At the opposite, if it has already access to its position, it will only have to check if its vertical and horizontal positions are greater, equals or smaller than those of the target. In standard RL, this problem is exacerbated, firstly because the only available learning process is the back-propagation of the reward signal, and secondly by the presence of noise in the raw state. It results that if the reward is sparse, the agent will not learn anything from its interactions even though interaction by themselves are rich in information. Furthermore, the state representation learned with a reward fully depends on the task and cannot be generalized to other tasks, whereas a state representation learned independently from the task can be used for other tasks.

Several works are about the learning of a relevant state representation. Auxiliary losses can complement the reward with supervised learning losses. It relies on information such as immediate reward or other predefined functions \cite{shelhamer2016loss,jaderberg2016reinforcement}. The agent may also use some prior knowledge on transitions \cite{jonschkowski2015learning,jonschkowski2017pves} or learn inverse models \cite{zhang2018decoupling}. There is a large literature on the best way to quickly build this kind of state space, we invite the interested reader to look at \cite{lesort2018state} for a general review and recommend \cite{bengio2013representation} for an introduction to the learning of representations. However, it is still difficult to get an entire disentangled representation of controllable objects since it can require interactions with the environment.

Although this issue did not attracted much attention, we will exhibit in Section \ref{sec:staterep} how IM can be a key component in order to build a state representation with such meaningful properties. We emphasize that we focus on works for which the intrinsic goal of the agent is to learn a \textit{state representation}. As a consequence, other ways to learn a \textit{state representation} are out of the scope of the section.

\subsection{Temporal abstraction of actions} \label{sec:abstraction}

Temporal abstraction of actions consists in using high-level actions, also called \textbf{options}, which can have different execution times \cite{sutton1999between}. Each option is associated with an \textbf{intra-option policy }which defines the action (low-level actions or other options) to realize in each state when the option is executed. The length of an option, which is the number of executed actions when an option is chosen, is often fixed. An \textbf{inter-option policy} can be in charge of choosing the options to accomplish. Abstract actions are a key element to accelerate the learning process since the number of decisions to take is significantly reduced if options are used. It also makes easier the \textit{credit assignment problem} \cite{sutton1998reinforcement}.
This problem refers to the fact that rewards can occur with a temporal delay and will only very weakly affect all temporally distant states that have preceded it, although these states may be important to obtain that reward. Indeed, the agent must propagate the reward along the entire sequence of actions (through Equation \eqref{eq:bellman}) to reinforce the first involved state-action tuple. This process can be very slow when the action sequence is large. This problem also concerns determining which action is decisive for getting the reward.

For example, let us assume that a robot is trying to reach a cake on a table which is far from the robot. If the robot has an option \texttt{get to the table} and follows it, the robot will then only have to take the cake to be rewarded. Then it will be easy to associate the acquisition of the cake (the reward) to the option \texttt{get to the table}. In contrast, if the robot has to learn to handle each of its joints (low-level or primitives actions), it will be difficult to determine which action is responsible of the acquisition of the cake, among all executed actions.%every actions executed. 

Furthermore, using options can make exploration easier when rewards are sparse, as illustrated in Figure \ref{im:abstract_actions}. The problem of exploration becomes trivial for the agent using options, since one exploration action can lead to the reward, yet it requires an entire sequence of specific low-level actions for the other agent. This problem arises from the minimal number of actions needed to get a reward. A thorough analysis of this aspect can be found in \cite{nachum2019does}.
\begin{figure}
\begin{centering}
\includegraphics[width=7cm]{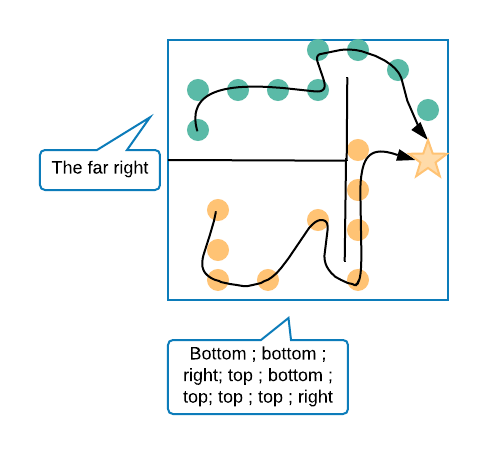}
\caption{Illustration of the benefits of using \textit{options}. Agents, represented by circles, have to reach the star. The green agent can use an \textit{option} \texttt{Go to the far right}; the orange agent can only use primitive actions to reach the star.}
\label{im:abstract_actions}
\end{centering}
\end{figure}

Regarding the intra-option policy, it can be manually defined, but it requires some extra expert knowledge \cite{sutton1999between}. It can also be learnt with the reward function \cite{bacon2017option,riemer2018learning}, but then, options are not reusable for other tasks and are helpless for the exploration problem.

In Section \ref{gen_goal}, we investigate how IM can bring new insights in handling this.

\subsection{Building a curriculum}

Curriculum learning commonly takes place in the framework of multi-task reinforcement learning \cite{WilsonFRT07,LiLC09} where one agent tries to solve several tasks. This is about defining a schedule in the learning process. It comes from the observation that learning is much easier when examples or tasks are organized in a meaningful order \cite{bengio2009curriculum}. Typically, a curriculum could organize tasks in such a way that they are increasingly complex and close to each other. For example, an helpful curriculum may be to first learn to a robot how to grasp a cube and only then how to move the cube; this way, the robot can take advantage of its ability to grasp a cube to move it. Without any prior knowledge, a robot would probably never succeed in grasping and moving a cube since it requires a large sequence of actions (if the robot moves its joints).

Standard methods rely on pre-specified tasks sequences as a curriculum \cite{karpathy2012curriculum}, or expert score which acts as a baseline score \cite{SharmaR17}. Some other methods require strong assumptions \cite{FlorensaHWZA17}, rely on task decomposition \cite{WuZS18} or availability of source tasks \cite{SvetlikLSSWS17,riedmiller2018learning}. It follows that most of the time in standard methods, \textit{curriculum learning} requires an expert in one way or another.

At the opposite, we will demonstrate in Section \ref{sec:curriculum} that it is possible to replace expert knowledge with IM to both speed up multi-task learning and indirectly make exploration easier.

\section{\textit{Empowerment}} \label{empowerment}

As presented in Section \ref{sect:background_empowerment}, an agent that maximizes empowerment tries to have the most control on its environment. To maximize empowerment in RL, the agent is rewarded if it is heading towards areas where it controls its environment. The intrinsic reward function is then defined as:
\begin{align}
    R_{int}(s,a,s') &= \Sigma(s') \nonumber \\
     & \approx -\mathbb{E}_{\omega (a|s)} \log \omega (a|s) + \mathbb{E}_{p(s'|a,s)\omega (a|s)}\log p(a|s,s') \label{eq:entropy2}. 
\end{align}

where $\omega (a|s)$ is the distribution choosing actions $a_t^n$. Ideally, $\omega (a|s)$ is the distribution maximizing Equation \eqref{eq:entropy2} in accordance with Equation \eqref{eq:meaning}.

The problem is that $p(a|s,s')$ is hard to obtain because it requires $p(s'|a,s)$ which is intractable. \\

\citename{mohamed2015variational} propose to compute the empowerment by approximating Equation \eqref{eq:entropy2}. To do this, they compute a lower bound of mutual information, used in many other works (Section \ref{miskill}):
\begin{equation}
    I(a;s'|s) \geq H(a|s) + \mathbb{E}_{p(s'|a,s)\omega (a|s)}\log q_{\xi}(a|s,s'). \label{eq:vlb}
\end{equation}

The idea is to learn an approximator $q_{\xi}$ of the probability distribution $p(a|s,s')$ in a supervised way with maximum likelihood method by using data received by the agent from its environment. This approach allows to generalize the computation of empowerment in order to process continuous observations. In this work, experiments show that the maximization of \textit{empowerment} is particularly useful in dynamic environments, i.e. environments where the agent's state can change even if the executed action is stationary (e.g. the agent does not move). The classic example provided in \citename{mohamed2015variational} is the prey-predator environment: the prey is the learner and tries to avoid to be caught as its death will cause a loss of control on the next states. Implicitly, the prey avoids to die by maximizing its \textit{empowerment}. In contrast to a dynamic environment, a static environment has a static optimal policy (the agent stops moving when it finds the best state) making \textit{empowerment} as an intrinsic reward less interesting according to a task. However, experiments proposed in \citename{mohamed2015variational} use planning methods to estimate \textit{empowerment} instead of interactions with the environment to collect data, which implies the use of a forward model.\\

\textbf{VIC} \cite{gregor2016variational} tries to maximize \textit{empowerment} with interactions with the environment using $\omega(a|s) = \pi(a|s)$. The intrinsic reward then becomes :
\begin{equation}
R_{int}(a,h) = -\log \pi(a|h) + \log \pi(a|s',h)
\end{equation}
where $h$ is the observation history (including current observation and action). The experiments on diverse environments show that learned trajectories lead to diverse areas and that a pretraining using \textit{empowerment} helps to learn a task. However, learned tasks are still relatively simple. The main issue may be that the \textit{empowerment} is hard to compute. We found few works related to \textit{empowerment} not following the formalism, while still rewarding the control of the agent.

Instead of directly using mutual information, \textbf{Mega-reward} \cite{song2019mega} cuts out the pixel space into a matrix which defines the probability of control of the corresponded part of the image. The intrinsic reward is then the matrix sum. They also show that the matrix can act as a mask to hide uncontrollable features, what other intrinsic exploration methods \cite{burda2018exploration} can benefit from to reduce the white-noise problem in a long-term way (as opposite to ICM method which detects short-term controllable features). However the method is inherently linked to pixel state environments. \citename{chuck2019hypothesis} provide a specific architecture relying on multiple assumptions such as the fact that an object can not spontaneously change its direction or its proximity to objects it interacts with. The agent formulates hypothesis on the \textit{controllability} of objects, which it tries to verify through a specific policy rewarded with an intrinsic verification process. Checked hypothesis can then be used directly as skills.\\

\textit{Empowerment} may also be interesting in multi-agents RL. Multi-agents RL is similar to mono-agent RL except that several agent learn simultaneously to solve a task and have to coordinate with each other. \citename{jaques2019social} show that in a non-cooperative game, as social dilemma \cite{leibo2017multi}, an \textit{empowerment}-based intrinsic reward could stabilize the learning process; the agent acts in order to influence other agents instead of looking for extrinsically rewarded behaviors. In fact, it compensates for the decrease of individual reward caused by a policy maximizing the long-term reward of all the agents.

To sum up, \textit{empowerment} is an interesting method to avoid an extrinsic reward and keep various complex behaviors. The main difficulty using \textit{empowerment} in RL is its complexity. Several approaches use an environment model to compute the reward based on \textit{empowerment} \cite{mohamed2015variational,de2018unified}. However the very essence of RL is that the agent does not know \textit{a priori} environment dynamics or the reward function. Existing work in this context remains relatively limited and is not sufficient to demonstrate the potential of \textit{empowerment} to help the learning process. It is interesting to note that \textit{empowerment} can push an agent to learn behaviors even in \textit{a priori} static environments. Indeed, let us assume that the agent does not choose primitive actions directly, but {options} instead. If it has not learned options, it will be unable to distinguish them, thus it is as if the agent had no control on the environment. On the contrary, if its options are perfectly distinguishable in the state space, the agent has control on its environment. In fact, the issue is not about choosing the states maximizing {empowerment}, but about defining options which increase overall \textit{empowerment}. We will come back to this point in Section \ref{gen_goal}.

\section{Intrinsic rewards with expert knowledge}\label{append:expert}

In this part, we will first study an article highlighting the promises of the approach, but relying on strong assumptions. Then we will describe some used heuristics which can not generalize to all environments.

\paragraph{Strong assumptions:}Seminal work shows the interest of decomposing hierarchically actions. Among them, \citename{kulkarni2016hierarchical} present the \textbf{hierarchical-DQN} in which the goal representation is expertly defined with tuples $(entity1,relation,entity2)$. An entity can be an object on the screen or an agent, and the relation notably refers to a distance. Therefore, the goal can be for the agent to reach an object. This reward is one if the goal is reached, zero otherwise. They show that it can help the learning process particularly when rewards are sparse like in \textit{Montezuma's revenge}. In fact, the more hierarchical the task is, the more required a hierarchical policy is \cite{complexity_exploration}.  However, by avoiding learning skill representation, \citename{kulkarni2016hierarchical} obfuscate the main problem: it is difficult to choose which features are interesting enough to be considered as goals in a large state space. 

\paragraph{Particular heuristics:} Other works demonstrate the potential of the approach using auxiliary objectives specific to the task \cite{riedmiller2018learning} or more abstract ones \cite{dilokthanakul2019feature,rafati2019unsupervised}. More particularly, an heuristic regularly used to generate skills is the search for the states acting as a bottleneck \cite{mcgovern2001automatic,menache2002q}. The main idea is to identify pivotal states relatively to the next visited states (e.g. a door). Recent works \cite{zhang2019scheduled,tomar2018successor} use successor representation \cite{kulkarni2016deep} to generalize the approach to continuous state space. Other heuristic can be the search for salient events \cite{barto2004intrinsically,chentanez2005intrinsically} such as changes in light. 

The limitation of this kind of works is that rewards are not sufficiently general to be applied in all environments. For example, there is no bottleneck state in an empty room whereas interesting skills can still be learned (going to the upper left corner).

\section{Simple goal sampling}\label{append:sampling}

Until now we have focused on IM as an intrinsic reward, however, this is not a general rule. For example, one can think of some simple strategies to choose tasks as long as the choice does not depend on an extrinsic reward. In this subsection, we study how such simple strategies can be efficient.

 \citename{andrychowicz2017hindsight} fully take advantage of \textbf{HER} and experimented different ways to sample goals on which to learn from trajectories. First the agent randomly sample a transition, then it replaces the initial goal by another one. They propose four strategies to choose the replacing goal:
\begin{itemize}
\item %The final state of the same episode as the transition being replayed.
The final state of the episode whose transition is being replayed.
\item Random goals originating from the episode whose transition is being replayed.%the same episode as the transition being replayed.
\item Sampling randomly from the buffer.
\item States arising after the transition being replayed in the same episode.
\end{itemize}

It appears that using future states or final states are the best working goals and generalization over the goal space pushes the agent towards its main goal. This is probably because these states act as a novelty bonus, helping the policy to generalize over the goal space and learn beyond its current abilities. In fact, count-based methods from Section \ref{sec:novelty} also reward the agent when it reaches a state it never went into: both methods have similar side-effects. The advantage of sampling methods compared to other contributions (\S\ref{sec:multi-armed} and \S\ref{sec:adversarial}) is that the agent continues to try to reach its true-goal state while performing exploration in the goal space. Few works extended HER while remaining in the field of IM. \textbf{Prioritized HER} \cite{zhao2019curiosity} proposes to adapt prioritized experience replay \cite{schaul2015prioritized} by over-weighting rare states. We can see this idea as an heuristic to consolidate novelty-based sampling. They slightly improve the results over HER at the cost of maintaining a density model. 

Even though these methods learn with new sampled goals, they act based on an extrinsic goal to solve. Therefore, they require a goal parameterized target. To improve exploration without an extrinsic parameterized goal, \textbf{UNICORN} \cite{mankowitz2018unicorn} samples uniformly in a goal space to interact with. This strategy can be effective since new goals and the generalization ability of the agent can make it go toward boundaries of its skills. However, it is unclear how the agent could behave in a poorly constructed goal space (such as a pixel state space).

\section{Review of tasks involving IM}\label{tasks}

We identified four fundamentally different types of tasks on which IM methods are tested. In this subsection we emphasize their particularities and the solving algorithm proposed in the literature.

\subsection{Locomotion}

Locomotion tasks are mostly related to MuJoCo environments such as \textit{ant} or \textit{humanoid} where the goal of the task is to move an agent \cite{duan2016benchmarking}. Most related work consider exploration and skill acquisition methods. Exploration methods only solve easy locomotion tasks, e.g. Half-Cheetah having a 17-dim observation space and 6-dim action space \cite{houthooft2016vime,pmlr-v97-kim19a,fu2017ex2}. On the other side, skill acquisition methods manage to learn to move forward (by crawling or walking) on harder morphologies, e.g. \textit{Ant} having a 111-dim observation space and a 8-dim action space \cite{achiam2018variational,eysenbach2018diversity}. Interestingly, a diversity heuristic without extrinsic reward suffices to get representations of different interesting skills. It suggests that diversity heuristic could be enough to handle proprioceptive incoming data. However, currently, too much useless skills are learnt and they can not be used while being learnt.

\subsection{Manipulation}\label{sec:manipulation}

Manipulation tasks can be about moving, pushing, reaching objects for a movable robotic arm. Few exploration methods have been tested \cite{lee2019efficient,pathak2019self} and they only manage to touch and move some objects. It is particularly interesting for skill acquisition methods \cite{hausman2018learning,nair2018visual} but this is not actually a major focus since it lacks object-oriented objective (as argued in \S\ref{sec:staterepr}). It is a standard task for\textit{curriculum learning}algorithms \cite{colas2019curious,santucci2019autonomous} since, for example, an agent has to learn to reach an item before moving it.\textit{curriculum learning}algorithms can be very efficient but at the cost of a hand-made goal space.

\subsection{Navigation}\label{sec:navigation}

Navigation tasks are about moving an agent in a maze. This is the broadly tested task and includes every kind of methods we presented. It can consist in moving a MuJoCo \textit{ant} or \textit{swimmer} in order to pick up food or to reach a target area. In the same way, Atari games generally consist in moving an agent into a rich environment, but with simpler discrete action space. Similarly to manipulation tasks, it requires target-oriented behaviors and favors the use of skills as states rather than diversity heuristic (despite a lot of progress in this way made by \citename{sharma2019dynamics}). Exploration methods are particularly efficient in discovering new areas and make sense, but are brute force and could be considerably improved as discussed in Sections \ref{sec:binding} and \ref{sec:staterepr}. Results of exploration through curriculum (\S\ref{curriculum_exploration}) also showed to be a nice alternative to standard exploration methods (\S\ref{sec:adversarial}) because of\textit{curriculum learning}capacity to capture different reward mode (\S\ref{im:detachment}).

\subsection{First-person view navigation}\label{sec:first_view}
First-person view navigation tasks are particularly challenging since the agent only receives a partial first-person visual view of its state and must learn its true state (e.g. its position). There are few work addressing these environments, mostly for exploration \cite{pathak2017curiosity,savinov2018episodic,fu2017ex2}, but they manage to efficiently explore the environment \cite{savinov2018episodic}. There is a lack of an application of count-based methods showing whether partial observability is a drag for the method. To the best of our knowledge, there is no work that tackle these environments in skill learning methods. It suggests a large need for a low-cost way to build the true state of the agent from partial observations. Yet, it is also not tackled in state representation learning methods.

Nevertheless, standard RL methods could take advantage of breaking down the partial observability into a long-term one at the higher level of the hierarchy, and into a short-term one at a lower level of the hierarchy. It could make the training of a recurrent neural network easier by reducing the gap between a notable event and the moment one needs to retrieve it in memory to get a reward. For example, in a 3D maze where the agent tries to reach an exit, a long-term memory could memorize large areas the agent went into whereas the short-term memory could focus on short time coherent behaviors.
